# Supplementary material for: Electric Multipoles of Double Majorana Kramers Pairs
Source: arXiv:2103.14398 ancillary file (2021-03-26)
Supplement: Supplementary file 1 [file supplemental.pdf]

# Supplemental Material: Electric Multipoles of Double Majorana Kramers Pairs

Yuki Yamazaki,[1] Shingo Kobayashi,[2] and Ai Yamakage[1]
[1]*Department of Physics, Nagoya University, Nagoya 464-8602, Japan*
[2]*RIKEN Center for Emergent Matter Science, Wako, Saitama 351-0198, Japan*

(Dated: March 26, 2021)

## CONTENTS

S1. Multipoles of double Majorana Kramers pairs and superconducting symmetry 1
A. Hamiltonian and symmetry 1
B. Multipole 1
C. Topological invariant 2
1. Winding number 2
2. $\mathbb{Z}_2$ invariant 2
3. Mirror reflection and twofold rotation 2
4. Threefold rotation 3
5. Four(Six)fold rotation 3
D. Irreducible representation of multipoles 3
1. $\mathbb{Z}_2$ invariant associated with threefold rotation 4
2. $pmg$, $\bar{X}_2 \oplus \bar{X}_5 \oplus \bar{X}_3 \oplus \bar{X}_4$ 4

S2. Antiperovskite 4
A. Model Hamiltonian 4
B. Symmetry operation 7
C. Strain 7

References 8

## S1. MULTIPOLES OF DOUBLE MAJORANA KRAMERS PAIRS AND SUPERCONDUCTING SYMMETRY

The main text has clarified the relation between the bulk superconducting symmetry, topological invariants, and electric multipoles of double Majorana Kramers pairs (MKPs) on the surface, which are coupled to strain. A general theory has been shown in the main text, but explicit results are given only for $p4m$ and $pg$ wallpaper groups (WGs). This section shows the results for all the WGs.

The strategy is as follows. List up all the possible topological invariants and bulk superconducting symmetry based on Table I in the main text. Next, determine electric multipoles of them from symmetry consideration, as done in the main text. Some of these cases do not need to be considered because of nonsymmorphic symmetry. To systematically take into account this property, we use a general scheme to obtain the irreducible decomposition of Majorana multipoles developed by Kobayashi et al. (Kobayashi *et al.*, 2020).

### A. Hamiltonian and symmetry

We start with an effective surface Majorana theory to make Supplemental Material self-contained. A Majorana field operator $\psi_i(\boldsymbol{x})$ satisfies the self-conjugate condition $\psi_i(\boldsymbol{x})^\dagger = \sum_j C_{ij}\psi_j(\boldsymbol{x})$ for $\boldsymbol{x} = (x, y)$ and $i, j = 1, \cdots, 2N$, where $C$ is a symmetric unitary matrix. $N = 2$ for double MKPs. The low-energy state around a time-reversal-invariant momentum (TRIM) is described by the Hamiltonian

$$H_{\rm surf} = \int d^2x \psi(\boldsymbol{x})^\dagger h_{\rm surf}(\boldsymbol{x})\psi(\boldsymbol{x}), \quad \text{(S1.1)}$$

with $h(\boldsymbol{x})$ the Hamiltonian density matrix. The above Hamiltonian must preserve particle-hole symmetry

$$\{\mathcal{C}, h_{\rm surf}(\boldsymbol{x})\} = 0,\ \mathcal{C} = C\mathcal{K}, \quad \text{(S1.2)}$$

with $\mathcal{K}$ the complex conjugation. Additionally we assume the theory respects time-reversal symmetry

$$[\mathcal{T}, h_{\rm surf}(\boldsymbol{x})] = 0,\ \mathcal{T} = (-is_y) \oplus \cdots \oplus (-is_y), \quad \text{(S1.3)}$$

where $s_i$ denotes the $i$th Pauli matrix acting on the spin space. The TRIM has the little-group $\mathcal{G}$ symmetry from a WG of the surface. The Hamiltonian must be invariant for $\psi(\boldsymbol{x}) \to D(g)^\dagger\psi(g\boldsymbol{x})$, $g \in \mathcal{G}$ as

$$D(g)h_{\rm surf}(\boldsymbol{x})D(g)^\dagger = h_{\rm surf}(g\boldsymbol{x}), \quad \text{(S1.4)}$$

where $D(g)$ denotes the representation matrix of $g$.

### B. Multipole

A physical observable of MKPs is given by

$$O_i(\boldsymbol{x}) = \psi(\boldsymbol{x})^\dagger\mathcal{O}_i(\boldsymbol{x})\psi(\boldsymbol{x}). \quad \text{(S1.5)}$$

$O_i(\boldsymbol{x})$ is decomposed into time-reversal-even (+, electric) and odd (−, magnetic) ones

$$O_i^\pm(\boldsymbol{x}) = \frac{O_i(\boldsymbol{x}) \pm \mathcal{T}O_i(\boldsymbol{x})\mathcal{T}^{-1}}{2}. \quad \text{(S1.6)}$$

$O_i^{\pm}(\boldsymbol{x})$ is decomposed into

$$O_i^{\pm}(\boldsymbol{x}) = \sum_A O_i^{A\pm}(\boldsymbol{x}), \tag{S1.7}$$

where $O_i^{A\pm}(\boldsymbol{x})$ belongs to an irrep of $\mathcal{G}$. Note that the electric monopole $O^{A+}(\boldsymbol{x})$ (totally symmetric irrep), including the charge density $\rho(\boldsymbol{x}) = \psi^\dagger(\boldsymbol{x})\psi(\boldsymbol{x})$, should be zero due to the charge neutrality of MKPs (Shiozaki and Sato, 2014). The irreducible decomposition of the magnetic multipoles $O^{A-}(\boldsymbol{x})$ for a single MKP was given exhaustively in (Kobayashi *et al.*, 2020). In the following we show the irreducible decomposition of the electromagnetic multipoles for double MKPs.

$O_i^{\pm}(\boldsymbol{x})$ is transformed by $g \in \mathcal{G}$ to

$$O_i^{\pm}(\boldsymbol{x}) \to \sum_j \mathcal{U}_{ij}^{\pm}(g) O_j^{\pm}(g\boldsymbol{x}). \tag{S1.8}$$

The character $\chi^{\pm}(g) = \mathrm{tr}\,\mathcal{U}^{\pm}(g)$ is calculated by the formula (Kobayashi *et al.*, 2020)

$$\chi^{\pm}(g) = \frac{\eta(g)}{4}\left(\Big\{\mathrm{tr}[D(g)]\Big\}^2 - \mathrm{tr}\big[D(g)^2\big]\right) \pm \frac{\eta(g)}{4}\left(\Big\{\mathrm{tr}[\Gamma D(g)]\Big\}^2 - \mathrm{tr}\Big[(\Gamma D(g))^2\Big]\right), \tag{S1.9}$$

where $\eta(g) = \pm 1$ is the character of $g$ for a one-dimensional irrep of the bulk pair potential, which is not explicitly given in the effective surface theory, and $\Gamma$ denotes the chiral operator defined by $\Gamma = i\mathcal{CT}$.

## C. Topological invariant

Both the bulk and surface Hamiltonians are block-diagonalized as $H^1 \oplus \cdots \oplus H^{|g|}$ in the $D(g)$ eigenspaces, where $|g|$ denotes the order of $g$. The $j$th eigenvalue of $D(g)$ is given by

$$\omega_j(g) = e^{-i(2j-1)\pi/|g|},\ j = 1, \cdots, |g|. \tag{S1.10}$$

### 1. Winding number

Chiral ($\Gamma$) and crystalline ($g$) symmetries define the winding number from the bulk Hamiltonian $H^i_{\mathrm{bulk}}(k_\perp)$. The momentum is along a high-symmetry line $(k_{x0}, k_{y0}, k_\perp)$, where $(k_{x0}, k_{y0})$ is a two-dimensional TRIM and $k_\perp$ is the component normal to the surface. The winding number is defined by (Wen and Zee, 1989)

$$w^i[g] = \frac{i}{4\pi}\int dk_\perp\, \mathrm{tr}\left(\Gamma^i H^{-1}_{\mathrm{bulk}}(k_\perp)\frac{\partial H^i_{\mathrm{bulk}}(k_\perp)}{\partial k_\perp}\right) \in \mathbb{Z}, \tag{S1.11}$$

$w^i[g]$ is quantized to an integer when $H^i_{\mathrm{bulk}}$ preserves the chiral symmetry, $\{\Gamma^i, H^i_{\mathrm{bulk}}\} = 0$, that is, the bulk pair potential is even parity ($\eta_g = 1$) for $g$, then $[\Gamma, D(g)] = 0$ holds (Ueno *et al.*, 2013). Furthermore, $w^i[g]$ can be nonzero when $H^i_{\mathrm{bulk}}$ breaks time-reversal symmetry $\omega_i(g)^* \neq \omega_i(g)$. The corresponding surface Hamiltonian $H^i_{\mathrm{surf}}$ hosts $|w^i[g]|$ Majorana fermions on the zero energy. It is the index theorem and bulk-boundary correspondence. Time-reversal symmetry ensures $\sum_{i=1}^{|g|} w^i[g] = 0$ hence the number of MKPs protected by the winding number of $g$ is given by

$$N[g] = \frac{1}{2}\sum_{i=1}^{|g|}\big|w^i[g]\big|. \tag{S1.12}$$

### 2. $\mathbb{Z}_2$ invariant

On the other hand, the $\mathbb{Z}_2$ invariant $\nu^i[g]$ from $H^i_{\mathrm{bulk}}$ is defined by

$$\nu^i[g] = \int \frac{dk_\perp}{2\pi} a^i, \tag{S1.13}$$

$$a^i = -i\sum_\alpha \sum_{s=\mathrm{I,II}} \langle k_\perp, i, \alpha, s|\frac{\partial\,|k_\perp, i, \alpha, s\rangle}{\partial k_\perp}, \tag{S1.14}$$

where $|k_\perp, i, \alpha, s\rangle$ is the $\alpha$th negative-energy state as

$$H^i_{\mathrm{bulk}}(k_\perp)\,|k_\perp, i, \alpha, s\rangle = -E_\alpha(k_\perp)\,|k_\perp, i, \alpha, s\rangle\,, \tag{S1.15}$$

for $E_\alpha(k_\perp) > 0$, and $s$ is the label for the Kramers partners I and II with the gauge fixing as

$$T^i\,|k_\perp, i, \alpha, \mathrm{I}\rangle = |-k_\perp, i, \alpha, \mathrm{II}\rangle\,, \tag{S1.16}$$

$$T^i\,|k_\perp, i, \alpha, \mathrm{II}\rangle = -\,|-k_\perp, i, \alpha, \mathrm{I}\rangle\,, \tag{S1.17}$$

with $T^i$ being the time reversal in the $i$th eigenspace, $T^i H^i_{\mathrm{bulk}}(k_\perp) T^{-1} = H^i_{\mathrm{bulk}}(-k_\perp)$. $\nu^i[g] \in \mathbb{Z}_2$ characterizes a zero-energy MKP in $H^i_{\mathrm{surf}}$ when $H^i$ preserves time-reversal symmetry $\omega_i(g)^* = \omega_i(g)$. If $\nu^i[g] = 1$ then $H^i_{\mathrm{surf}}$ hosts a single MKP (Sato *et al.*, 2011).

In the subsequent sections, we show how to determine the winding number from the surface theory for each case. $\mathbb{Z}_2$ invariants, on the other hand, are deduced from the winding numbers and the irreducible decomposition of multipoles. The detail shall be shown in Sec S1.D.2.

### 3. Mirror reflection and twofold rotation

For $g$ a mirror reflection or a twofold rotation, the winding number of $g$ is expressed in (Xiong *et al.*, 2017)

$$w^1[g] - w^2[g] = \frac{i}{4\pi}\int dk_\perp \times \mathrm{tr}\left(i\Gamma D(g) H_{\mathrm{bulk}}(k_\perp)^{-1}\frac{\partial H_{\mathrm{bulk}}(k_\perp)}{\partial k_\perp}\right). \tag{S1.18}$$

In the surface theory, on the other hand, zero-energy states are eigenstates of the chiral operator with the eigenvalues (chiralities) $\pm 1$. The index theorem tells us that this chirality equals $w^i[g]$ obtained in the bulk theory (Sato *et al.*, 2011). As a result, we have the bulk-boundary correspondence

$$\mathrm{tr}(i\Gamma D(g))_{\mathrm{surf}} = i\sum_{i=1}^{|g|} w^i[g]\omega_i(g) = 2w^1[g]. \tag{S1.19}$$

The number of MKPs protected by the winding number of $g$ is given by

$$N[g] = \frac{1}{2}|\mathrm{tr}(i\Gamma D(g))_{\mathrm{surf}}|. \tag{S1.20}$$

### 4. Threefold rotation

For $g = C_3$ threefold rotation, both the bulk and surface Hamiltonians in the basis diagonalizing $D(C_3)$ are expressed as

$$H^1 \oplus H^2 \oplus H^3, \tag{S1.21}$$

where $H^j$ is in the $D(C_3) = \omega_j(C_3) = e^{-i(2j-1)\pi/3}$ eigenspace. $H^1$ is the Kramers partner of $H^3$ because of $\omega_1(C_3)^* = \omega_3(C_3)$. $H^2$ is time-reversal-invariant by itself. Therefore one has

$$w^1[C_3] + w^3[C_3] = w^2[C_3] = 0. \tag{S1.22}$$

The number of MKPs protected by the winding number of $C_3$ is given by

$$N[C_3] = \big|w^1[C_3]\big|, \tag{S1.23}$$

and

$$\mathrm{tr}(\Gamma D(C_3))_{\mathrm{surf}} = -i\sqrt{3}w^1[C_3], \tag{S1.24}$$

or

$$N[C_3] = \frac{1}{\sqrt{3}}|\mathrm{tr}(\Gamma D(C_3))_{\mathrm{surf}}|, \tag{S1.25}$$

thanks to $w^2[C_3] = 0$.

On the one hand, $H^2$ respects time-reversal symmetry $\omega_2(C_3)^* = \omega_2(C_3)$ and has no winding number but the $\mathbb{Z}_2$ invariant $\nu^2[C_3]$. Instead of calculating the $\mathbb{Z}_2$ topological invariant $\nu^2[C_3]$ directly in the surface theory, they can be obtained from the relationship between the electric multipoles and the winding numbers. An example will be given in Sec. S1.D.1.

### 5. Four(Six)fold rotation

For fourfold rotation $C_4$, time-reversal symmetry $[\omega_1(C_4)^* = \omega_4(C_4)$ and $\omega_2(C_4)^* = \omega_3(C_4)]$ requires

$$w^1[C_4] + w^4[C_4] = w^2[C_4] + w^3[C_4] = 0. \tag{S1.26}$$

Therefore we have

$$\begin{aligned}\mathrm{tr}(\Gamma D(C_4))_{\mathrm{surf}} &= \sum_{i=1}^{4} w^i[C_4]\omega_i(C_4) \\ &= -i\sqrt{2}\big(w^1[C_4] + w^2[C_4]\big).\end{aligned} \tag{S1.27}$$

Simultaneously we have the relation for the twofold rotation $D(C_2) = D(C_4)^2$ as

$$\begin{aligned}\mathrm{tr}(\Gamma D(C_2))_{\mathrm{surf}} = \mathrm{tr}\big(\Gamma D(C_4)^2\big)_{\mathrm{surf}} &= \sum_{i=1}^{4} w^i[C_4]\omega_i(C_4)^2 \\ &= -i2\big(w^1[C_4] - w^2[C_4]\big).\end{aligned} \tag{S1.28}$$

Consequently, the number of MKPs protected by the winding number of $C_4$ is given by

$$\begin{aligned}N[C_4] =& \left|\frac{1}{2\sqrt{2}}\mathrm{tr}(\Gamma D(C_4))_{\mathrm{surf}} + \frac{1}{4}\mathrm{tr}(\Gamma D(C_2))_{\mathrm{surf}}\right| \\ &+ \left|\frac{1}{2\sqrt{2}}\mathrm{tr}(\Gamma D(C_4))_{\mathrm{surf}} - \frac{1}{4}\mathrm{tr}(\Gamma D(C_2))_{\mathrm{surf}}\right|.\end{aligned} \tag{S1.29}$$

The number of MKPs protected by the winding number of sixfold rotation $C_6$ is obtained in a similar way. The result is given by

$$\begin{aligned}N[C_6] =& \left|\frac{1}{6}\mathrm{tr}(\Gamma D(C_6))_{\mathrm{surf}} + \frac{\sqrt{3}}{6}\mathrm{tr}(\Gamma D(C_3))_{\mathrm{surf}}\right. \\ &\left. + \frac{1}{6}\mathrm{tr}(\Gamma D(C_2))_{\mathrm{surf}}\right| \\ &+ \left|\frac{1}{3}\mathrm{tr}(\Gamma D(C_6))_{\mathrm{surf}} - \frac{1}{6}\mathrm{tr}(\Gamma D(C_2))_{\mathrm{surf}}\right| \\ &+ \left|\frac{1}{6}\mathrm{tr}(\Gamma D(C_6))_{\mathrm{surf}} - \frac{\sqrt{3}}{6}\mathrm{tr}(\Gamma D(C_3))_{\mathrm{surf}}\right. \\ &\left. + \frac{1}{6}\mathrm{tr}(\Gamma D(C_2))_{\mathrm{surf}}\right|.\end{aligned} \tag{S1.30}$$

## D. Irreducible representation of multipoles

Now we are in a position to discuss the irreducible decomposition of multipoles of double MKPs. The results are shown in Tables S1 and S2. The following summarizes the procedure for the irreducible decomposition of the Majorana multipoles.

1. Set a WG of the surface, TRIM, the corresponding little group $\mathcal{G} \subset$ WG, and irrep of bulk pair potential $\Delta$.

2. Set a representation $\bar{X}$ of double ($N = 2$) MKPs. Physical (time-reversal-invariant) double-valued irreps for WGs are found in Bilbao Crystallographic Server (Elcoro *et al.*, 2017). Two cases: (1) Direct sum of two time-reversal-invariant two-dimensional irreps $X = \bar{A}_1 \oplus \bar{A}_2$, including $\bar{A}_1 = \bar{A}_2$. (2) One time-reversal-invariant four-dimensional irrep $\bar{X}$, which is realized in nonsymmorphic cases.

3. Write down the $4 \times 4$ representation matrix of $g$, $D(g)$, for the double MKPs $\bar{X}$. Irreps of $g$ are also found in Bilbao Crystallographic Server.

4. Construct the charge conjugation $\mathcal{C} = C\mathcal{K}$. $C$ is a symmetric unitary matrix and satisfies

$$[\mathcal{C}, D(g)] = 0, \quad \text{for} \quad \eta(g) = 1, \tag{S1.31}$$
$$\{\mathcal{C}, D(g)\} = 0, \quad \text{for} \quad \eta(g) = -1. \tag{S1.32}$$

   The chiral operator is obtained by $\Gamma = i\mathcal{C}\mathcal{T}$. In some cases, the representation of the chiral operator is not uniquely determined, and each may give different topological invariants and multipoles. An example is shown in S1.D.2.

5. Calculate Eq. (S1.9) and decompose it into irreps of the point group compatible with WG. If the result includes an electric totally symmetric irrep, which contradicts the charge neutrality, there is no MKP.

We comment on some exceptional cases.

### 1. $\mathbb{Z}_2$ invariant associated with threefold rotation

$\bar{\Gamma}_4$ [with $D(C_3) = \omega_2(C_3) = -1$] of $p3$ is a one-dimensional double-valued real irrep (Elcoro *et al.*, 2017), which does not preserve time-reversal symmetry. As a result, $2\bar{\Gamma}_4$ is a time-reversal-invariant irrep and hosts no winding number of $C_3$ but the $\mathbb{Z}_2$ invariant $\nu^2[C_3] = 1$. Besides, $\bar{\Gamma}_5 \oplus \bar{\Gamma}_6$ yields a single MKP associated with $N[C_3] = \sqrt{3}^{-1} |\,\mathrm{tr}(\Gamma D(C_3))_{\mathrm{surf}}| = 1$. Namely,

$$N[C_3] = \nu^2[C_3] = 1. \tag{S1.33}$$

The same situation is realized in the double MKPs of $\bar{\Gamma}_4 \oplus \bar{\Gamma}_5 \oplus \bar{\Gamma}_6$ for $p31m$, $\bar{\Gamma}_7 \oplus \bar{\Gamma}_8 \oplus \bar{\Gamma}_{10} \oplus \bar{\Gamma}_{11}$ for $p6$, $\bar{\Gamma}_7 \oplus \bar{\Gamma}_8 \oplus \bar{\Gamma}_9 \oplus \bar{\Gamma}_{12}$ for $p6$, $\bar{\Gamma}_7 \oplus \bar{\Gamma}_9$ for $p6m$, and $\bar{\Gamma}_7 \oplus \bar{\Gamma}_8$ for $p6m$.

### 2. $pmg$, $\bar{X}_2 \oplus \bar{X}_5 \oplus \bar{X}_3 \oplus \bar{X}_4$

$pmg$ is Abelian on the $X$ point. The winding number and $\mathbb{Z}_2$ invariant can simultaneously protect double MKPs. Actually, for double MKPs of $\bar{X}_2 \oplus \bar{X}_5 \oplus \bar{X}_3 \oplus \bar{X}_4$, there are two cases of the topological invariants, $N[m_{10}] = 2$ & $\nu^1[g_{01}] = \nu^2[g_{01}] = 1$ or $N[C_2] = 2$ & $\nu^1[g_{01}] = \nu^2[g_{01}] = 1$, each with a different electric multipole, $2A_2$ or $2B_2$, respectively. This distinction stems from the nonuniqueness of representations of the chiral operator $\Gamma$.

Here we show how to determine the $\mathbb{Z}_2$ invariant, considering $pmg$, $A_1$, $\bar{X}_2 \oplus \bar{X}_5 \oplus \bar{X}_3 \oplus \bar{X}_4$, and $N[m_{10}] = 2$, $\nu^1[g_{01}] = \nu^2[g_{01}] = 1$, as an example. The number and irrep of electric multipoles of MKPs protected by the winding number of $m_{10}$ have been extracted by the procedure given above, $N[m_{10}] = 2$ and $2A_2$, respectively. However, if the double MKPs are protected by $N[m_{10}] = 2$ and $\nu^1[g_{01}] = \nu^2[g_{01}] = 0$, $B_1$ electric perturbations, which break $m_{10}$ symmetry, are coupled to them, i.e., double MKPs have to host $B_1$ electric multipoles in addition to $A_2$. Resolving this contradiction, the double MKPs must be protected by $N[m_{10}] = 2$ and $\nu^1[g_{01}] = \nu^2[g_{01}] = 1$, for which the double MKPs are robust against $B_1$ perturbations. Thus, the $\mathbb{Z}_2$ invariants are deduced from the relationship between the winding numbers and the electric multipoles. The same situation occurs for $p4g$.

## S2. ANTIPEROVSKITE

This section shows a model of antiperovskite and its symmetry.

### A. Model Hamiltonian

The BdG Hamiltonian for an antiperovskite with the $A_{1u}$ pairing used in the main text has the form (Kawakami *et al.*, 2018)

$$H_{\mathrm{bulk}}(\boldsymbol{k}) = h(\boldsymbol{k}) + \Delta_0 \sigma_x \tau_x, \tag{S2.1}$$
$$h(\boldsymbol{k}) = \left[-m_0 + \alpha \sum_i \{2 - 2\cos(k_i)\}\right]\sigma_z + \sin\boldsymbol{k} \cdot \left(v_1 \boldsymbol{J} + v_2 \tilde{\boldsymbol{J}}\right)\sigma_x - \mu\sigma_0. \tag{S2.2}$$

Here, $\boldsymbol{J}$ and $\tilde{\boldsymbol{J}}$ are $4 \times 4$ matrices of spin–3/2 and represented as

$$J_x = \frac{1}{2}\begin{pmatrix} 0 & \sqrt{3} & 0 & 0 \\ \sqrt{3} & 0 & 2 & 0 \\ 0 & 2 & 0 & \sqrt{3} \\ 0 & 0 & \sqrt{3} & 0 \end{pmatrix}, \tag{S2.3}$$

$$J_y = \frac{i}{2}\begin{pmatrix} 0 & -\sqrt{3} & 0 & 0 \\ \sqrt{3} & 0 & -2 & 0 \\ 0 & 2 & 0 & -\sqrt{3} \\ 0 & 0 & \sqrt{3} & 0 \end{pmatrix}, \tag{S2.4}$$

$$J_z = \frac{1}{2}\begin{pmatrix} 3 & 0 & 0 & 0 \\ 0 & 1 & 0 & 0 \\ 0 & 0 & -1 & 0 \\ 0 & 0 & 0 & -3 \end{pmatrix}, \tag{S2.5}$$

and $\tilde{J}_i \equiv \frac{5}{3}\sum_{j \neq i} J_j J_i J_j - \frac{7}{6} J_i$ given by

TABLE S1 Electromagnetic degrees of freedom of double Majorana Kramers pairs (MKPs). They emerge on the surface with wallpaper-group (WG) symmetry, when the bulk pair potential belongs to irrep $\Delta$. Irreps of double MKPs, electric operators of MKPs, which couple to strain [$u_{ij}(\boldsymbol{x}) = \partial_i u_j(\boldsymbol{x})$, where $\boldsymbol{u}(\boldsymbol{x})$ denotes the displacement field], are also shown. We adapt the definition for WG and irreps by Bilbao Crystallographic Server (Elcoro *et al.*, 2017). $\bar{\Gamma}_i$ denotes the $i$th double-valued irrep of the little group on the $\Gamma$ point. $2\bar{\Gamma}_i = \bar{\Gamma}_i \oplus \bar{\Gamma}_i$. Octupole $O_i$ is defined by $O_x = \partial_x u_{xx} - \partial_x u_{yy} - \partial_y u_{xy} - \partial_y u_{yx}$ and $O_y = \partial_y u_{yy} - \partial_y u_{xx} - \partial_x u_{yx} - \partial_x u_{xy}$. The result for $P3m1$ are the same as that for $P31m$.

| WG | $\Delta$ | MKPs | Topo | Electric | Strain | Magnetic |
|---|---|---|---|---|---|---|
| $p2$ | $A$ | $2(\bar{\Gamma}_3 \oplus \bar{\Gamma}_4)$ | $N[C_2] = 2$ | $2B$ | $u_{xz}$, $u_{zx}$, $u_{yz}$, $u_{zy}$ | $4A$ |
| $p3$ | $A$ | $2(\bar{\Gamma}_5 \oplus \bar{\Gamma}_6)$ | $N[C_3] = 2$ | $E$ | $(u_{xx} - u_{yy}, u_{xy} + u_{yx})$, $(u_{xz}, u_{yz})$, $(u_{zx}, u_{zy})$ | $4A$ |
| $p3$ | $A$ | $2\bar{\Gamma}_4 \oplus \bar{\Gamma}_5 \oplus \bar{\Gamma}_6$ | $N[C_3] = \nu^2[C_3] = 1$ | $E$ | $(u_{xx} - u_{yy}, u_{xy} + u_{yx})$, $(u_{xz}, u_{yz})$, $(u_{zx}, u_{zy})$ | $2A + E$ |
| $p4$ | $A$ | $2(\bar{\Gamma}_5 \oplus \bar{\Gamma}_7)$, $2(\bar{\Gamma}_6 \oplus \bar{\Gamma}_8)$ | $N[C_4] = N[C_2] = 2$ | $E$ | $(u_{xz}, u_{yz})$, $(u_{zx}, u_{zy})$ | $4A$ |
| $p4$ | $A$ | $\bar{\Gamma}_5 \oplus \bar{\Gamma}_7 \oplus \bar{\Gamma}_6 \oplus \bar{\Gamma}_8$ | $N[C_4] = N[C_2] = 2$ | $E$ | $(u_{xz}, u_{yz})$, $(u_{zx}, u_{zy})$ | $2A + 2B$ |
| $p4$ | $A$ | $\bar{\Gamma}_5 \oplus \bar{\Gamma}_7 \oplus \bar{\Gamma}_6 \oplus \bar{\Gamma}_8$ | $N[C_4] = 2$ | $2B$ | $(u_{xx} - u_{yy}, u_{xy} + u_{yx})$ | $2A + E$ |
| $p6$ | $A$ | $2(\bar{\Gamma}_7 \oplus \bar{\Gamma}_8)$ | $N[C_6] = N[C_2] = 2$ | $2B$ | $O_x$, $O_y$ | $4A$ |
| $p6$ | $A$ | $2(\bar{\Gamma}_9 \oplus \bar{\Gamma}_{12})$, $2(\bar{\Gamma}_{10} \oplus \bar{\Gamma}_{11})$ | $N[C_6] = N[C_3] = N[C_2] = 2$ | $E_1$ | $(u_{xz}, u_{yz})$, $(u_{zx}, u_{zy})$ | $4A$ |
| $p6$ | $A$ | $\bar{\Gamma}_7 \oplus \bar{\Gamma}_8 \oplus \bar{\Gamma}_9 \oplus \bar{\Gamma}_{12}$, $\bar{\Gamma}_7 \oplus \bar{\Gamma}_8 \oplus \bar{\Gamma}_{10} \oplus \bar{\Gamma}_{11}$ | $N[C_6] = N[C_2] = 2$, $N[C_3] = \nu^2[C_3] = 1$ | $E_1$ | $(u_{xz}, u_{yz})$, $(u_{zx}, u_{zy})$ | $2A + E_2$ |
| $p6$ | $A$ | $\bar{\Gamma}_7 \oplus \bar{\Gamma}_8 \oplus \bar{\Gamma}_9 \oplus \bar{\Gamma}_{12}$, $\bar{\Gamma}_7 \oplus \bar{\Gamma}_8 \oplus \bar{\Gamma}_{10} \oplus \bar{\Gamma}_{11}$ | $N[C_6] = W[C_3] = 2$, $N[C_3] = \nu^2[C_3] = 1$ | $E_2$ | $(u_{xx} - u_{yy}, u_{xy} + u_{yx})$ | $2A + E_1$ |
| $p6$ | $A$ | $\bar{\Gamma}_9 \oplus \bar{\Gamma}_{12} \oplus \bar{\Gamma}_{10} \oplus \bar{\Gamma}_{11}$ | $N[C_6] = N[C_2] = 2$ | $2B$ | $O_x$, $O_y$ | $2A + E_2$ |
| $p6$ | $A$ | $\bar{\Gamma}_9 \oplus \bar{\Gamma}_{12} \oplus \bar{\Gamma}_{10} \oplus \bar{\Gamma}_{11}$ | $N[C_6] = N[C_3] = 2$ | $E_2$ | $(u_{xx} - u_{yy}, u_{xy} + u_{yx})$ | $2A + 2B$ |
| $pm$ | $A'$ | $2(\bar{\Gamma}_3 \oplus \bar{\Gamma}_4)$ | $N[m_{10}] = 2$ | $2A''$ | $u_{xy}$, $u_{yx}$, $u_{yz}$, $u_{zy}$ | $4A'$ |
| $pmm$ | $A_2$ | $2\bar{\Gamma}_5$ | $N[C_2] = 2$ | $B_1 + B_2$ | $u_{xz}$, $u_{zx}$, $u_{yz}$, $u_{zx}$ | $4A_2$ |
| $pmm$ | $B_1$ | $2\bar{\Gamma}_5$ | $N[m_{01}] = 2$ | $A_2 + B_2$ | $u_{xy}$, $u_{yx}$, $u_{yz}$, $u_{zy}$ | $4B_1$ |
| $pmm$ | $B_2$ | $2\bar{\Gamma}_5$ | $N[m_{10}] = 2$ | $A_2 + B_1$ | $u_{xy}$, $u_{yx}$, $u_{xz}$, $u_{zx}$ | $4B_2$ |
| $p31m$ | $A_1$ | $2(\bar{\Gamma}_4 \oplus \bar{\Gamma}_5)$ | $N[m_{1\bar{1}}] = N[m_{12}] = N[m_{21}] = 2$ | $2A_2$ | $u_{xy} - u_{yx}$ | $4A_1$ |
| $p31m$ | $A_2$ | $2\bar{\Gamma}_6$ | $N[C_3] = 2$ | $E$ | $(u_{xx} - u_{yy}, u_{xy} + u_{yx})$, $(u_{xz}, u_{yz})$, $(u_{zx}, u_{zy})$ | $A_1 + 3A_2$ |
| $p31m$ | $A_2$ | $\bar{\Gamma}_4 \oplus \bar{\Gamma}_5 \oplus \bar{\Gamma}_6$ | $N[C_3] = \nu^2[C_3] = 1$ | $E$ | $(u_{xx} - u_{yy}, u_{xy} + u_{yx})$, $(u_{xz}, u_{yz})$, $(u_{zx}, u_{zy})$ | $2A_2 + E$ |
| $p4m$ | $A_2$ | $2\bar{\Gamma}_6$, $2\bar{\Gamma}_7$ | $N[C_4] = N[C_2] = 2$ | $E$ | $(u_{xz}, u_{yz})$, $(u_{zx}, u_{zy})$ | $A_1 + 3A_2$ |
| $p4m$ | $A_2$ | $\bar{\Gamma}_6 \oplus \bar{\Gamma}_7$ | $N[C_4] = N[C_2] = 2$ | $E$ | $(u_{xz}, u_{yz})$, $(u_{zx}, u_{zy})$ | $2A_2 + B_1 + B_2$ |
| $p4m$ | $A_2$ | $\bar{\Gamma}_6 \oplus \bar{\Gamma}_7$ | $N[C_4] = 2$ | $B_1 + B_2$ | $u_{xx} - u_{yy}$, $u_{xy} + u_{yx}$ | $2A_2 + E$ |
| $p6m$ | $A_2$ | $2\bar{\Gamma}_8$, $2\bar{\Gamma}_9$ | $N[C_6] = N[C_3] = N[C_2] = 2$ | $E_1$ | $u_{xz}$, $u_{zx}$, $u_{yz}$, $u_{zy}$ | $A_1 + 3A_2$ |
| $p6m$ | $A_2$ | $2\bar{\Gamma}_7$ | $N[C_6] = N[C_2] = 2$ | $B_1 + B_2$ | $O_x$, $O_y$ | $A_1 + 3A_2$ |
| $p6m$ | $A_2$ | $\bar{\Gamma}_7 \oplus \bar{\Gamma}_9$, $\bar{\Gamma}_7 \oplus \bar{\Gamma}_8$ | $N[C_6] = N[C_2] = 2$, $N[C_3] = \nu^2[C_3] = 1$ | $E_1$ | $(u_{xz}, u_{yz})$, $(u_{zx}, u_{zy})$ | $2A_2 + E_2$ |
| $p6m$ | $A_2$ | $\bar{\Gamma}_7 \oplus \bar{\Gamma}_9$, $\bar{\Gamma}_7 \oplus \bar{\Gamma}_8$ | $N[C_6] = 2$, $N[C_3] = \nu^2[C_3] = 1$ | $E_2$ | $(u_{xx} - u_{yy}, u_{xy} + u_{yx})$ | $2A_2 + E_1$ |
| $p6m$ | $A_2$ | $\bar{\Gamma}_8 \oplus \bar{\Gamma}_9$ | $N[C_6] = N[C_2] = 2$ | $B_1 + B_2$ | $O_x$, $O_y$ | $2A_2 + E_2$ |
| $p6m$ | $A_2$ | $\bar{\Gamma}_8 \oplus \bar{\Gamma}_9$ | $N[C_6] = N[C_3] = 2$ | $E_2$ | $(u_{xx} - u_{yy}, u_{xy} + u_{yx})$ | $2A_2 + B_1 + B_2$ |
| $p6m$ | $B_1$ | $2\bar{\Gamma}_7$ | $N[m_{1\bar{1}}] = N[m_{12}] = N[m_{21}] = 2$ | $A_2 + B_2$ | $u_{xy} - u_{yx}$, $O_y$ | $A_1 + 3B_1$ |
| $p6m$ | $B_2$ | $2\bar{\Gamma}_7$ | $N[m_{11}] = N[m_{10}] = N[m_{01}] = 2$ | $A_2 + B_1$ | $u_{xy} - u_{yx}$, $O_x$ | $A_1 + 3B_2$ |

TABLE S2 Continued from Table S1 for nonsymmorphic WGs. $\bar{B}_i$, $\bar{X}_i$, $\bar{S}_i$, and $\bar{M}_i$ are double-valued irrep of the little group on the $B$, $X$, $S$, and $M$ points, defined in Bilbao Crystallographic Server (Elcoro *et al.*, 2017), respectively.

| WG | $\Delta$ | MKPs | Topo | Electric | Strain | Magnetic |
|---|---|---|---|---|---|---|
| $pg$ | $A'$ | $2\bar{B}_3 \oplus 2\bar{B}_4$ | $\nu^1[g_{01}] = \nu^2[g_{01}] = 1$ | $2A''$ | $u_{xy}$, $u_{yx}$, $u_{yz}$, $u_{zy}$ | $2A' + 2A''$ |
| $pmg$ | $A_1$ | $2(\bar{X}_2 \oplus \bar{X}_5)$, $2(\bar{X}_3 \oplus \bar{X}_4)$ | $N[C_2] = N[m_{10}] = 2$ | $2B_1$ | $u_{xz}$, $u_{zx}$ | $4A_1$ |
| $pmg$ | $A_1$ | $\bar{X}_2 \oplus \bar{X}_5 \oplus \bar{X}_3 \oplus \bar{X}_4$ | $N[m_{10}] = 2$, $\nu^1[g_{01}] = \nu^2[g_{01}] = 1$ | $2A_2$ | $u_{xy}$, $u_{yx}$ | $2A_1 + 2B_2$ |
| $pmg$ | $A_1$ | $\bar{X}_2 \oplus \bar{X}_5 \oplus \bar{X}_3 \oplus \bar{X}_4$ | $N[C_2] = 2$, $\nu^1[g_{01}] = \nu^2[g_{01}] = 1$ | $2B_2$ | $u_{yz}$, $u_{zy}$ | $2A_1 + 2A_2$ |
| $pmg$ | $B_1$ | $\bar{X}_2 \oplus \bar{X}_5 \oplus \bar{X}_3 \oplus \bar{X}_4$ | $\nu^1[g_{01}] = \nu^2[g_{01}] = 1$ | $A_2 + B_2$ | $u_{xy}$, $u_{yx}$, $u_{yz}$, $u_{zy}$ | $A_2 + 2B_1 + B_2$ |
| $pgg$ | $A_1$ | $2\bar{S}_5$ | $\nu^1[g_{01}] = \nu^2[g_{01}]$ $= \nu^1[g_{10}] = \nu^2[g_{10}] = 1$ | $2A_2$ | $u_{xy}$, $u_{yx}$ | $A_1 + A_2 + B_1 + B_2$ |
| $pgg$ | $A_2$ | $2\bar{S}_5$ | $N[C_2] = 2$ | $B_1 + B_2$ | $u_{xz}$, $u_{zx}$, $u_{yz}$, $u_{zy}$ | $3A_1 + A_2$ |
| $pgg$ | $B_1$ | $2\bar{S}_5$ | $\nu^1[g_{01}] = \nu^2[g_{01}] = 1$ | $A_2 + B_2$ | $u_{xy}$, $u_{yx}$, $u_{yz}$, $u_{zy}$ | $A_1 + B_1 + 2B_2$ |
| $pgg$ | $B_2$ | $2\bar{S}_5$ | $\nu^1[g_{10}] = \nu^2[g_{10}] = 1$ | $A_2 + B_1$ | $u_{xy}$, $u_{yx}$, $u_{xz}$, $u_{zy}$ | $A_1 + 2B_1 + B_2$ |
| $p4g$ | $A_1$ | $\bar{M}_6 \oplus \bar{M}_7$ | $N[C_4] = 2$, $\nu^1[g_{10}] = \nu^2[g_{10}]$ $= \nu^1[g_{01}] = \nu^2[g_{01}] = 1$ | $2B_2$ | $u_{xy} + u_{yx}$ | $A_1 + A_2 + E$ |
| $p4g$ | $A_2$ | $\bar{M}_6 \oplus \bar{M}_7$ | $N[C_4] = N[C_2] = 2$ | $E$ | $(u_{xz}, u_{yz})$, $(u_{zx}, u_{zy})$ | $A_1 + A_2 + 2B_1$ |
| $p4g$ | $B_1$ | $\bar{M}_6 \oplus \bar{M}_7$ | $\nu^1[g_{10}] = \nu^2[g_{10}]$ $= \nu^1[g_{01}] = \nu^2[g_{01}] = 1$ | $A_2 + B_2$ | $u_{xy} - u_{yx}$, $u_{xy} + u_{yx}$ | $A_2 + B_1 + E$ |

$$\tilde{J}_x = \frac{1}{4}\begin{pmatrix} 0 & \sqrt{3} & 0 & -5 \\ \sqrt{3} & 0 & -3 & 0 \\ 0 & -3 & 0 & \sqrt{3} \\ -5 & 0 & \sqrt{3} & 0 \end{pmatrix}, \tag{S2.6}$$

$$\tilde{J}_y = \frac{i}{4}\begin{pmatrix} 0 & -\sqrt{3} & 0 & -5 \\ \sqrt{3} & 0 & 3 & 0 \\ 0 & -3 & 0 & -\sqrt{3} \\ 5 & 0 & \sqrt{3} & 0 \end{pmatrix}, \tag{S2.7}$$

$$\tilde{J}_z = \frac{1}{2}\begin{pmatrix} -1 & 0 & 0 & 0 \\ 0 & 3 & 0 & 0 \\ 0 & 0 & -3 & 0 \\ 0 & 0 & 0 & 1 \end{pmatrix}. \tag{S2.8}$$

$\sigma_0$ and $\sigma_i$ denotes the identity and $i$th Pauli matrix, respectively, which dictate the orbital parity.

## B. Symmetry operation

Antiperovskites have the $O_h$ point group symmetry. For convenience, irreps of the generators ($2_{001}$, $2_{010}$, $3^+_{111}$, $2_{110}$, and $\bar{1}$, where we adapt the notation used in Bilbao Crystallographic Server) are shown in Table S3.

The symmetry operations in the model space are represented by $8\times 8$ matrices, which are complicated. However, in practice, as in (Kawakami *et al.*, 2018), the Pauli matrices $\sigma_\mu$ and spin-3/2 matrices $\boldsymbol{J}$ and $\tilde{\boldsymbol{J}}$ are enough to construct models, order parameters, and external perturbations, from symmetry consideration. Interestingly, $\boldsymbol{J}$ and $\tilde{\boldsymbol{J}}$ have the same irreducible decomposition as the angular momentum so that we can regard them as the angular momentum under $O_h$ symmetry, which serves a simple and universal viewpoint.

$\sigma_0$ and $\sigma_z$ are scalars, $\sigma_x$ is a pseudoscalar, and $\sigma_y$ is also a pseudoscalar but with broken time-reversal symmetry (Kawakami *et al.*, 2018). Hence they are decomposed into irreps of $O_h$, as summarized in Table S4. By referring to Table S4 only, we can efficiently obtain an arbitrary physical quantity belonging to an irrep by irreducible decomposition for the product of those listed there. As given in the following, the Hamiltonian induced by strain is obtained in this way.

## C. Strain

Unsymmetrized strain tensor $u_{ij}$ is defined by $u_{ij} = \partial_i u_j$ with $\boldsymbol{u}$ the lattice displacement field. They are coupled to squares of angular momenta. Due to the symmetry constraint, from Table S4, the coupling Hamiltonian between static strain and angular momentum in the zero order of momentum, which is invariant against the transform of $u_{ij}$ and $J_k$ by the symmetry operation, is given by the linear combination of the direct products of $\sigma_\mu$ ($\mu = 0,\, z$) and

$$u_{xx} + u_{yy} + u_{zz}, \tag{S2.9}$$

$$(2u_{zz} - u_{xx} - u_{yy})\left(2J_z^2 - J_x^2 - J_y^2\right) + 3(u_{xx} - u_{yy})\left(J_x^2 - J_y^2\right), \tag{S2.10}$$

$$(u_{xy} - u_{yx})(J_xJ_y + J_yJ_x) + (u_{yz} - u_{zy})(J_yJ_z + J_zJ_y) + (u_{zx} - u_{xz})(J_zJ_x + J_xJ_z). \tag{S2.11}$$

$\sigma_x$ and $\sigma_y$ are spatial-inversion odd (pseudoscalar) and not coupled to the strain, which is spatial-inversion even. Note that the $T_{1g}$ irrep $(J_z, J_x, J_y)$ is not directly coupled to strain because it breaks time-reversal symmetry, while a dynamical strain can be coupled as $(\dot{u}_{xy} - \dot{u}_{yx})J_z + (\dot{u}_{yz} - \dot{u}_{zy})J_x + (\dot{u}_{zx} - \dot{u}_{xz})J_y = \boldsymbol{\nabla} \times \dot{\boldsymbol{u}} \cdot \boldsymbol{J}$, which is nothing but the spin(−3/2)–vorticity coupling (Matsuo *et al.*, 2013).

TABLE S3 Even-parity irreducible representations (Irrep) of the generators of $O_h$. The notation defined in Bilbao Crystallographic Server (Aroyo *et al.*, 2006) is used for symmetry operations and irreps. $E_g$ irrep is given in a basis different from Bilbao Crystallographic Server.

| Irrep | $2_{001}$ | $2_{010}$ | $3^+_{111}$ | $2_{110}$ | $\bar{1}$ |
|---|---|---|---|---|---|
| $A_{1g}$ | 1 | 1 | 1 | 1 | 1 |
| $A_{2g}$ | 1 | 1 | 1 | −1 | 1 |
| $E_g$ | $\begin{pmatrix}1&0\\0&1\end{pmatrix}$ | $\begin{pmatrix}1&0\\0&1\end{pmatrix}$ | $\begin{pmatrix}-1/2&-\sqrt{3}/2\\\sqrt{3}/2&-1/2\end{pmatrix}$ | $\begin{pmatrix}1&0\\0&-1\end{pmatrix}$ | $\begin{pmatrix}1&0\\0&1\end{pmatrix}$ |
| $T_{1g}$ | $\begin{pmatrix}1&0&0\\0&-1&0\\0&0&-1\end{pmatrix}$ | $\begin{pmatrix}-1&0&0\\0&-1&0\\0&0&1\end{pmatrix}$ | $\begin{pmatrix}0&0&1\\1&0&0\\0&1&0\end{pmatrix}$ | $\begin{pmatrix}-1&0&0\\0&0&1\\0&1&0\end{pmatrix}$ | $\begin{pmatrix}1&0&0\\0&1&0\\0&0&1\end{pmatrix}$ |
| $T_{2g}$ | $\begin{pmatrix}1&0&0\\0&-1&0\\0&0&-1\end{pmatrix}$ | $\begin{pmatrix}-1&0&0\\0&-1&0\\0&0&1\end{pmatrix}$ | $\begin{pmatrix}0&0&1\\1&0&0\\0&1&0\end{pmatrix}$ | $\begin{pmatrix}1&0&0\\0&0&-1\\0&-1&0\end{pmatrix}$ | $\begin{pmatrix}1&0&0\\0&1&0\\0&0&1\end{pmatrix}$ |

TABLE S4 Irreducible decomposition of $\sigma_\mu$, angular momentum, and strain. The same holds for $\tilde{\boldsymbol{J}}$.

| Irrep | Parity | Angular momentum | Strain |
|---|---|---|---|
| $A_{1g}$ | $\sigma_0$, $\sigma_z$ | 1 | $u_{xx}+u_{yy}+u_{zz}$ |
| $E_g$ | | $(2J_z^2-J_x^2-J_y^2, -\sqrt{3}(J_x^2-J_y^2))$ | $(2u_{zz}-u_{xx}-u_{yy}, -\sqrt{3}(u_{xx}-u_{yy}))$ |
| $T_{1g}$ | | $(J_z, J_x, J_y)$ | $(u_{xy}-u_{yx}, u_{yz}-u_{zy}, u_{zx}-u_{xz})$ |
| $T_{2g}$ | | $(J_xJ_y+J_yJ_x, J_yJ_z+J_zJ_y, J_zJ_x+J_xJ_z)$ | $(u_{xy}+u_{yx}, u_{yz}+u_{zy}, u_{zx}+u_{xz})$ |
| $A_{1u}$ | $\sigma_x$, $\sigma_y$ | | |

## REFERENCES


Aroyo, Mois I, Asen Kirov, Cesar Capillas, J. M. Perez-Mato, and Hans Wondratschek (2006), "Bilbao Crystallographic Server. II. Representations of crystallographic point groups and space groups," Acta Cryst. **A62** (2), 115–128.

Elcoro, Luis, Barry Bradlyn, Zhijun Wang, Maia G. Vergniory, Jennifer Cano, Claudia Felser, B. Andrei Bernevig, Danel Orobengoa, Gemma de la Flor, and Mois I. Aroyo (2017), "Double crystallographic groups and their representations on the Bilbao Crystallographic Server," J Appl. Cryst. **50** (5), 1457–1477.

Kawakami, Takuto, Tetsuya Okamura, Shingo Kobayashi, and Masatoshi Sato (2018), "Topological Crystalline Materials of $J = 3/2$ Electrons: Antiperovskites, Dirac Points, and High Winding Topological Superconductivity," Phys. Rev. X **8**, 041026.

Kobayashi, Shingo, Yuki Yamazaki, Ai Yamakage, and Masatoshi Sato (2020), arXiv:2011.06770.

Matsuo, Mamoru, Jun'ichi Ieda, Kazuya Harii, Eiji Saitoh, and Sadamichi Maekawa (2013), "Mechanical generation of spin current by spin-rotation coupling," Phys. Rev. B **87**, 180402.

Sato, Masatoshi, Yukio Tanaka, Keiji Yada, and Takehito Yokoyama (2011), "Topology of Andreev bound states with flat dispersion," Phys. Rev. B **83**, 224511.

Shiozaki, Ken, and Masatoshi Sato (2014), "Topology of crystalline insulators and superconductors," Phys. Rev. B **90**, 165114.

Ueno, Yuji, Ai Yamakage, Yukio Tanaka, and Masatoshi Sato (2013), "Symmetry-Protected Majorana Fermions in Topological Crystalline Superconductors: Theory and Application to $Sr_2RuO_4$," Phys. Rev. Lett. **111**, 087002.

Wen, XG, and A. Zee (1989), "Winding number, family index theorem, and electron hopping in a magnetic field," Nucl. Phys. B **316** (3), 641–662.

Xiong, Yuansen, Ai Yamakage, Shingo Kobayashi, Masatoshi Sato, and Yukio Tanaka (2017), "Anisotropic Magnetic Responses of Topological Crystalline Superconductors," Crystals **7** (2), 58.
